# Supplementary material for: Structure and Overlaps of Communities in Networks
Source: arXiv:1205.6228 source file (2012-09-25)
Supplement: Supplementary file 1 [file 070appendix.tex]

\xhdr{Edge clustering in community overlaps}
We further analyze  how connectivity patterns of nodes in the overlap differ from node connectivity patterns in the non-overlapping part of the community. We conduct the following experiment. For every node $u$ in the overlap $O$, we first identify which of $u$'s neighbors belong to only $A$ (but not $B$), only  $B$ (but not $A$), and which to the overlap $O$. Let's denote these sets of nodes as $A_u$, $B_u$ and $O_u$.
%\rev{Strictly speaking, $A_u$, $B_u$ are $A_u \setminus O_u$, $B_u \setminus O_u$ as the nodes in $A_u$ or $B_u$ do not belong to $O$, but we choose these notations for simplicity.}
We then compute $XY(u)$ which denotes the fraction of connected pairs of nodes $x \in X$ and $y \in Y$ (where $X, Y$ is one of $A_u, B_u,O_u$).
For example, $OO(u)$ denotes the fraction of edges that are present among $u$'s neighbors that are in the overlap. In other words $OO(u)$ is the clustering coefficient~\cite{watts98collective} of the overlap. Similarly, $AB(u)$ is the ``cross-community'' clustering where one neighbor of $u$ is in $A_u$ and the other in $B_u$, and $AABB(u)$ is the ``in-community'' clustering. For example, in Figure~\ref{fig:overlap.toy}, all the neighbors of $u$ that are in $O$ are connected with each other so $OO(u)=1$, Whereas, two out of three pairs of nodes in $A$ are connected, and there are no connections between neighbors in $B$, so $AABB(u)=2/4=0.5$. Since no nodes in $A$ are connected to nodes in $B$, $AB(u)=0$.

\begin{figure*}[t]
	\centering
	\subfigure[LJ]{\includegraphics[width=0.31\textwidth]{OverlapCCF.lj.eps}}
    \subfigure[Friendster]{\includegraphics[width=0.31\textwidth]{OverlapCCF.friendster.eps}}
	\subfigure[Orkut]{\includegraphics[width=0.31\textwidth]{OverlapCCF.orkut.eps}}
	\subfigure[DBLP]{\includegraphics[width=0.31\textwidth]{OverlapCCF.dblp.eps}}
	\subfigure[IMDB]{\includegraphics[width=0.31\textwidth]{OverlapCCF.imdbc.eps}}
	\subfigure[Amazon]{\includegraphics[width=0.31\textwidth]{OverlapCCF.amazon.eps}}
  \vspace{-4mm}
	\caption{The average fraction of the connected pairs of neighbors as a function of node degree. AABB: both neighbors in either $A$ or $B$, OO: both neighbors in overlap $O$, AB: one neighbor in $A$ and the other in $B$.}
  \vspace{-4mm}
\label{fig:full.overlap.triangle}
\end{figure*}

Figure~\ref{fig:full.overlap.triangle} plots average $OO(u)$, $AABB(u)$, and $AB(u)$ as a function of the degree of $u$. We observe that the nodes in the community overlap are more densely connected than the nodes that only belong to a single community as $OO(u)$ is generally higher than $AABB(u)$. $AB(u)$ exhibits lower values than either of $AABB(u)$ and $OO(u)$, which suggests that nodes that belong to different communities are less likely to form connections. Notice similar behavior for all six datasets, where connections are most likely to be formed if the nodes belong to the overlap (red curve), less likely if they both belong to the same community (green curve) and least likely if the pair of nodes belongs to different communities (blue curve).

%In this experiment, we considered all the neighbors of a node to compute the
%clustering coefficient. So, multi membership nodes have high CCF not because
%overlap $O$ is dense, but because their neighbors in $A$, $B$ and elsewhere are
%connected among themselves. To disambiguate this, we conducted the following
%experiment. For every node $u$ in $O$, we first identify which of $u$'s
%neighbors belong $A$, $B$, and which to the overlap $O$. Let's denote these
%nodes as $A_u$, $B_u$ and $O_u$. We then compute $XY(u)$ which denotes the
%fraction connected pairs of nodes $x \in X$ and $y \in Y$ (and $X,Y$ is one of
%$A_u, B_u,O_u$).
%
%we computed the fraction of two neighbors in $O$ (between red nodes) are
%connected each other, and denote it by $OO(u)$.
%
%For the same node $u$, we measured the fraction of neighbors in A or neighbors
%in B (between green nodes or between blue nodes) that are connected, and call
%it $AABB(u)$. Finally, we also examined the same quantity for a pair between a
%green and a blue node, and denote it by $AB(u)$.

\xhdr{Community size and membership distribution}
Figure~\ref{fig:Full.Sz.CCDF} and \ref{fig:Full.Mem.CCDF} show the distribution of community size and node memberships in the 6 networks with ground-truth communities.
\begin{figure*}[t]
	\centering
    \subfigure[LiveJournal]{\includegraphics[width=0.31\textwidth]{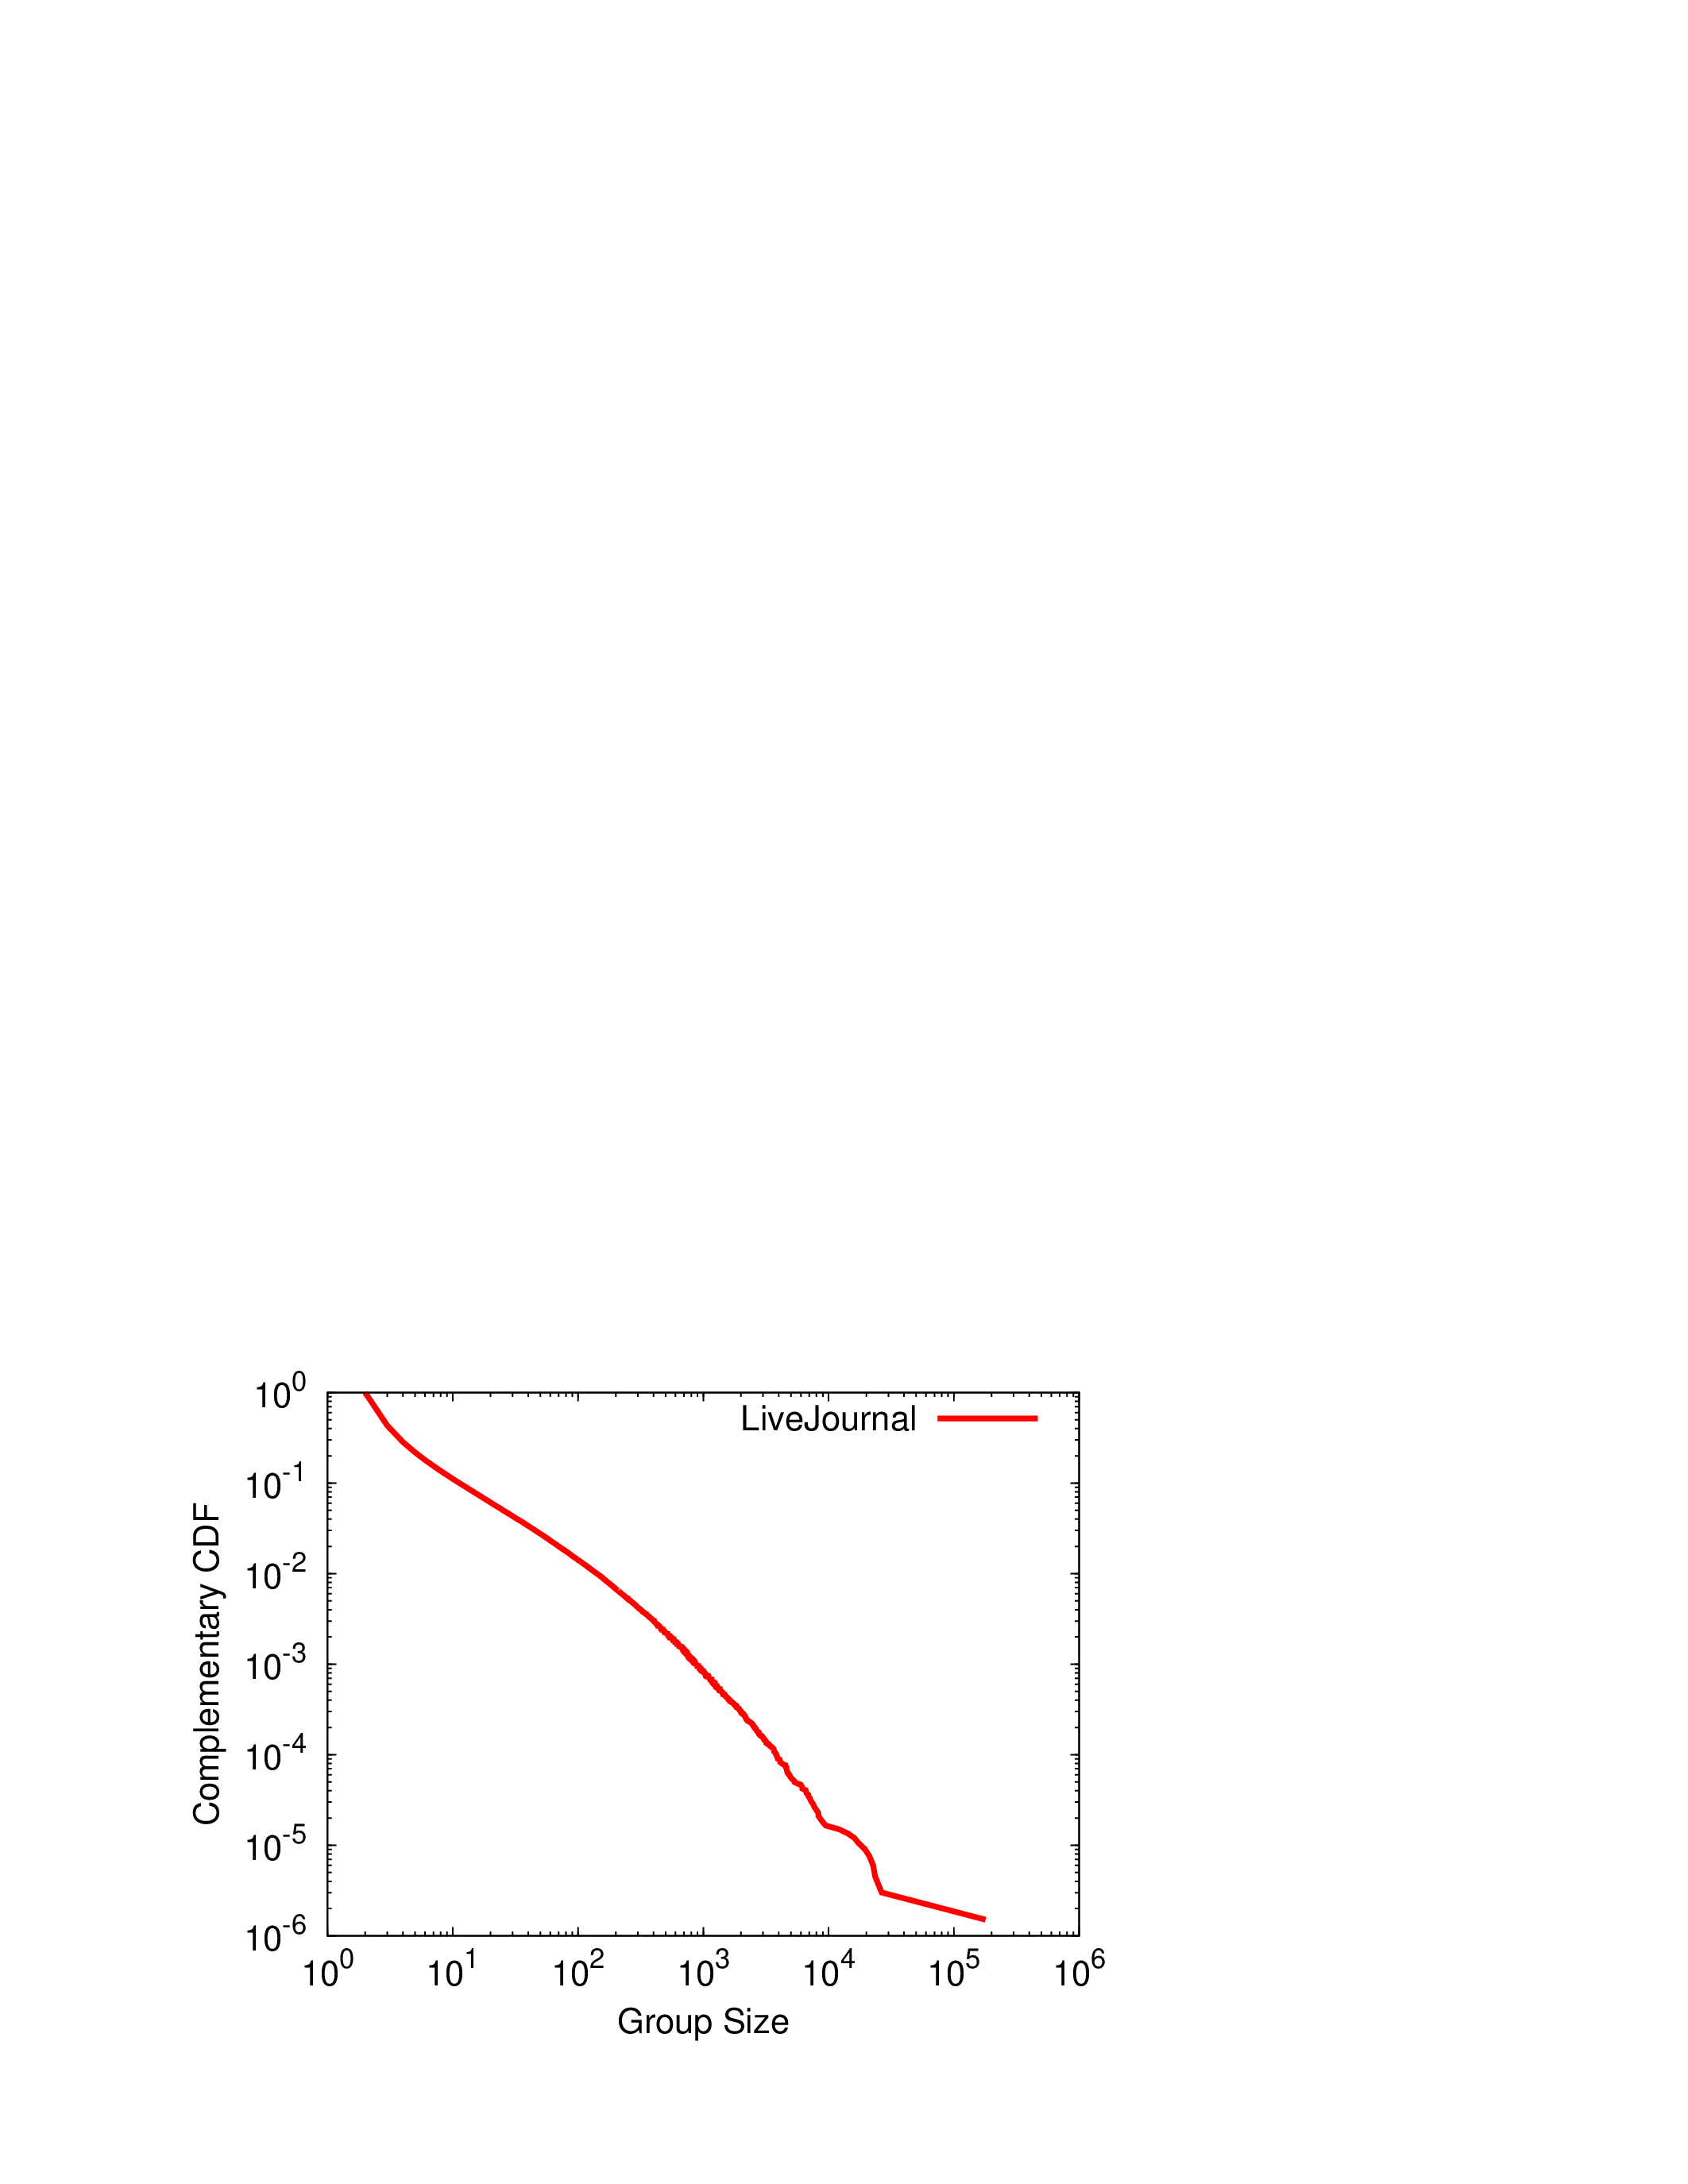}}
	\subfigure[Friendster]{\includegraphics[width=0.31\textwidth]{Sz_Dist_friendster.eps}}
	\subfigure[Orkut]{\includegraphics[width=0.31\textwidth]{Sz_Dist_orkut.eps}}\\
	\subfigure[DBLP]{\includegraphics[width=0.31\textwidth]{Sz_Dist_dblp.eps}}
	\subfigure[IMDB]{\includegraphics[width=0.31\textwidth]{Sz_Dist_imdbc.eps}}
    \subfigure[Amazon]{\includegraphics[width=0.31\textwidth]{Sz_Dist_amazon.eps}}
	\caption{
    \textbf{Community size distribution.}
    Complementary cumulative distribution function $F_c(s)$ of the size of ground-truth communities, $s$. The size of a community denotes the number of nodes belonging to the community.
    }
\label{fig:Full.Sz.CCDF}
\end{figure*}

\begin{figure*}[t]
	\centering
    \subfigure[LiveJournal]{\includegraphics[width=0.31\textwidth]{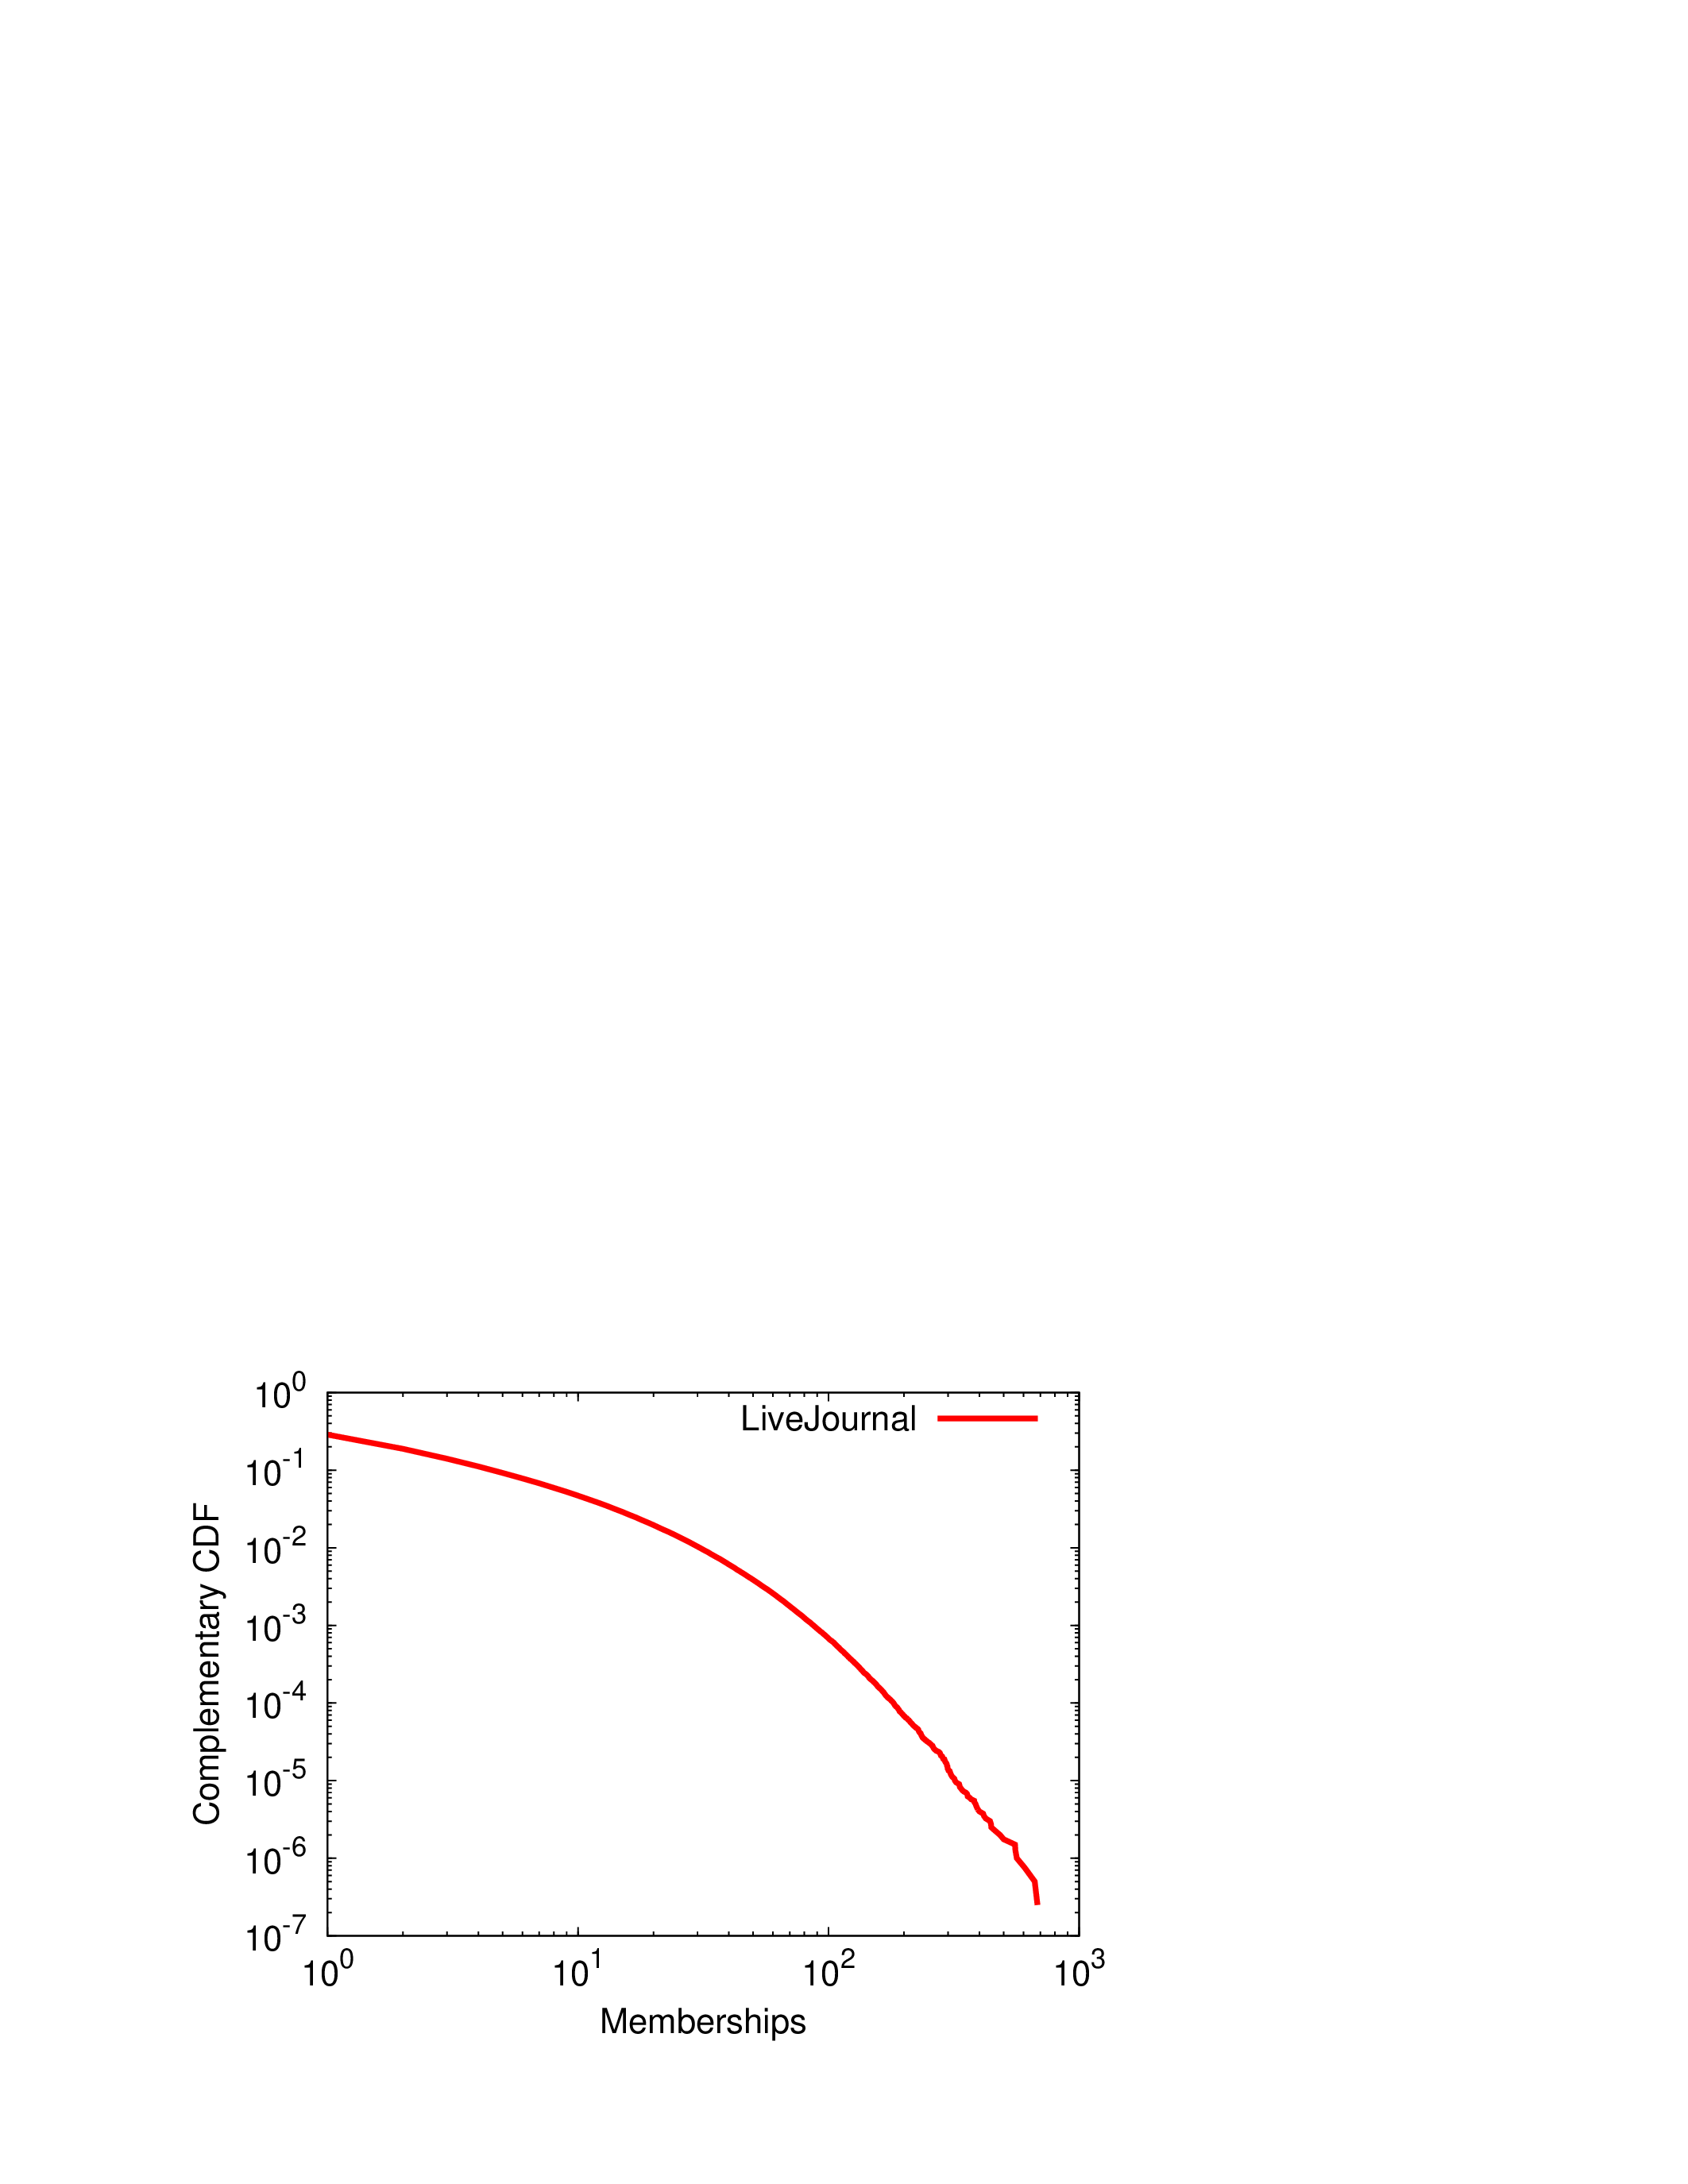}}
	\subfigure[Friendster]{\includegraphics[width=0.31\textwidth]{Mem_Dist_friendster.eps}}
	\subfigure[Orkut]{\includegraphics[width=0.31\textwidth]{Mem_Dist_orkut.eps}}\\
	\subfigure[DBLP]{\includegraphics[width=0.31\textwidth]{Mem_Dist_dblp.eps}}
	\subfigure[IMDB]{\includegraphics[width=0.31\textwidth]{Mem_Dist_imdbc.eps}}
    \subfigure[Amazon]{\includegraphics[width=0.31\textwidth]{Mem_Dist_amazon.eps}}
	\caption{
    \textbf{Membership size distribution.}
    Complementary cumulative distribution function $F_c(m)$ of the node memberships $m$. Memberships of a node mean the number of communities that the node belong to.
    }
\label{fig:Full.Mem.CCDF}
\end{figure*}

\xhdr{Model comparison}
Figure~\ref{fig:Full.Models.Groupstats} shows the group properties modeled by \agm and LFR. Figure~\ref{fig:Full.Models.edge_prob} and \ref{fig:Full.hub.overlap.models} show the properties of overlaps modeled by \agm and LFR.
\begin{figure*}[t]
	\centering
	\subfigure[Edges inside	 (LJ)]{\includegraphics[width=0.16\textwidth]{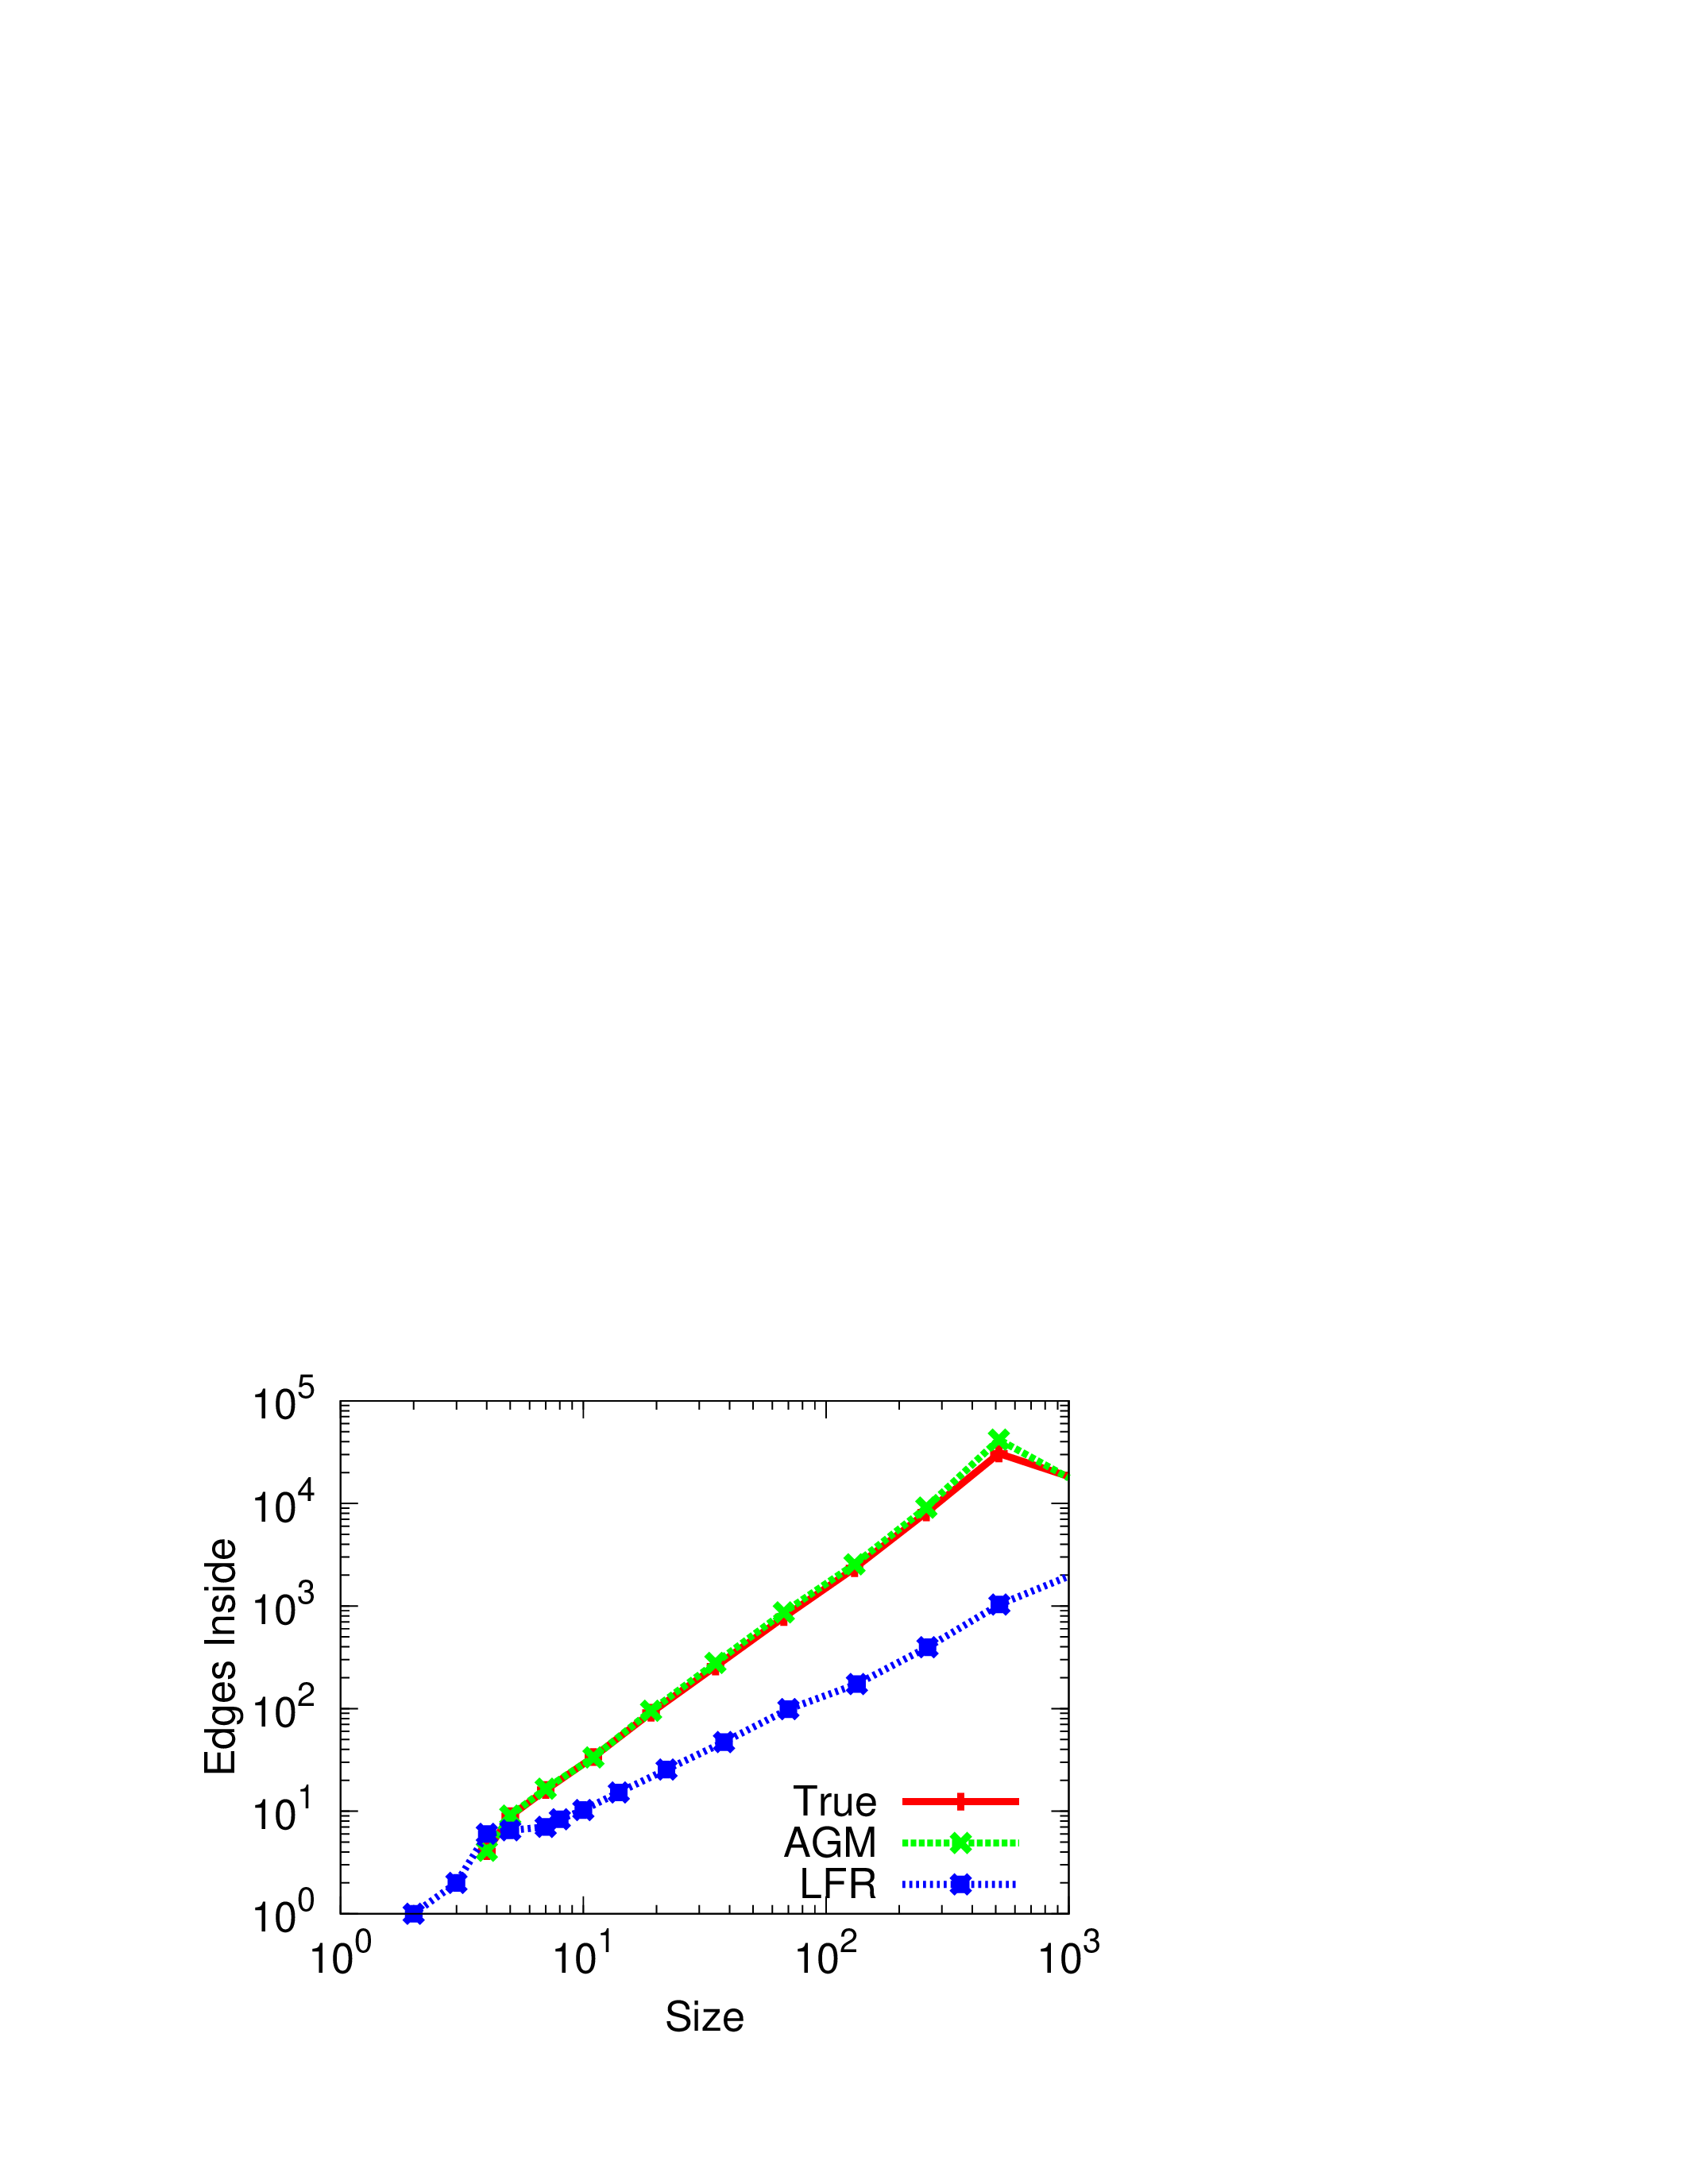}}
	\subfigure[Edges inside	 (Friendster)]{\includegraphics[width=0.16\textwidth]{Models.P.Sz.Vol.friendster.eps}}
	\subfigure[Edges inside	 (Orkut)]{\includegraphics[width=0.16\textwidth]{Models.P.Sz.Vol.orkut.eps}}
	\subfigure[Edges inside	 (DBLP)]{\includegraphics[width=0.16\textwidth]{Models.P.Sz.Vol.dblp.eps}}
	\subfigure[Edges inside	 (IMDB)]{\includegraphics[width=0.16\textwidth]{Models.P.Sz.Vol.imdbc.eps}}
	\subfigure[Edges inside	 (Amazon)]{\includegraphics[width=0.16\textwidth]{Models.P.Sz.Vol.amazon.eps}}
	\subfigure[Maximum ICDF	 (LJ)]{\includegraphics[width=0.16\textwidth]{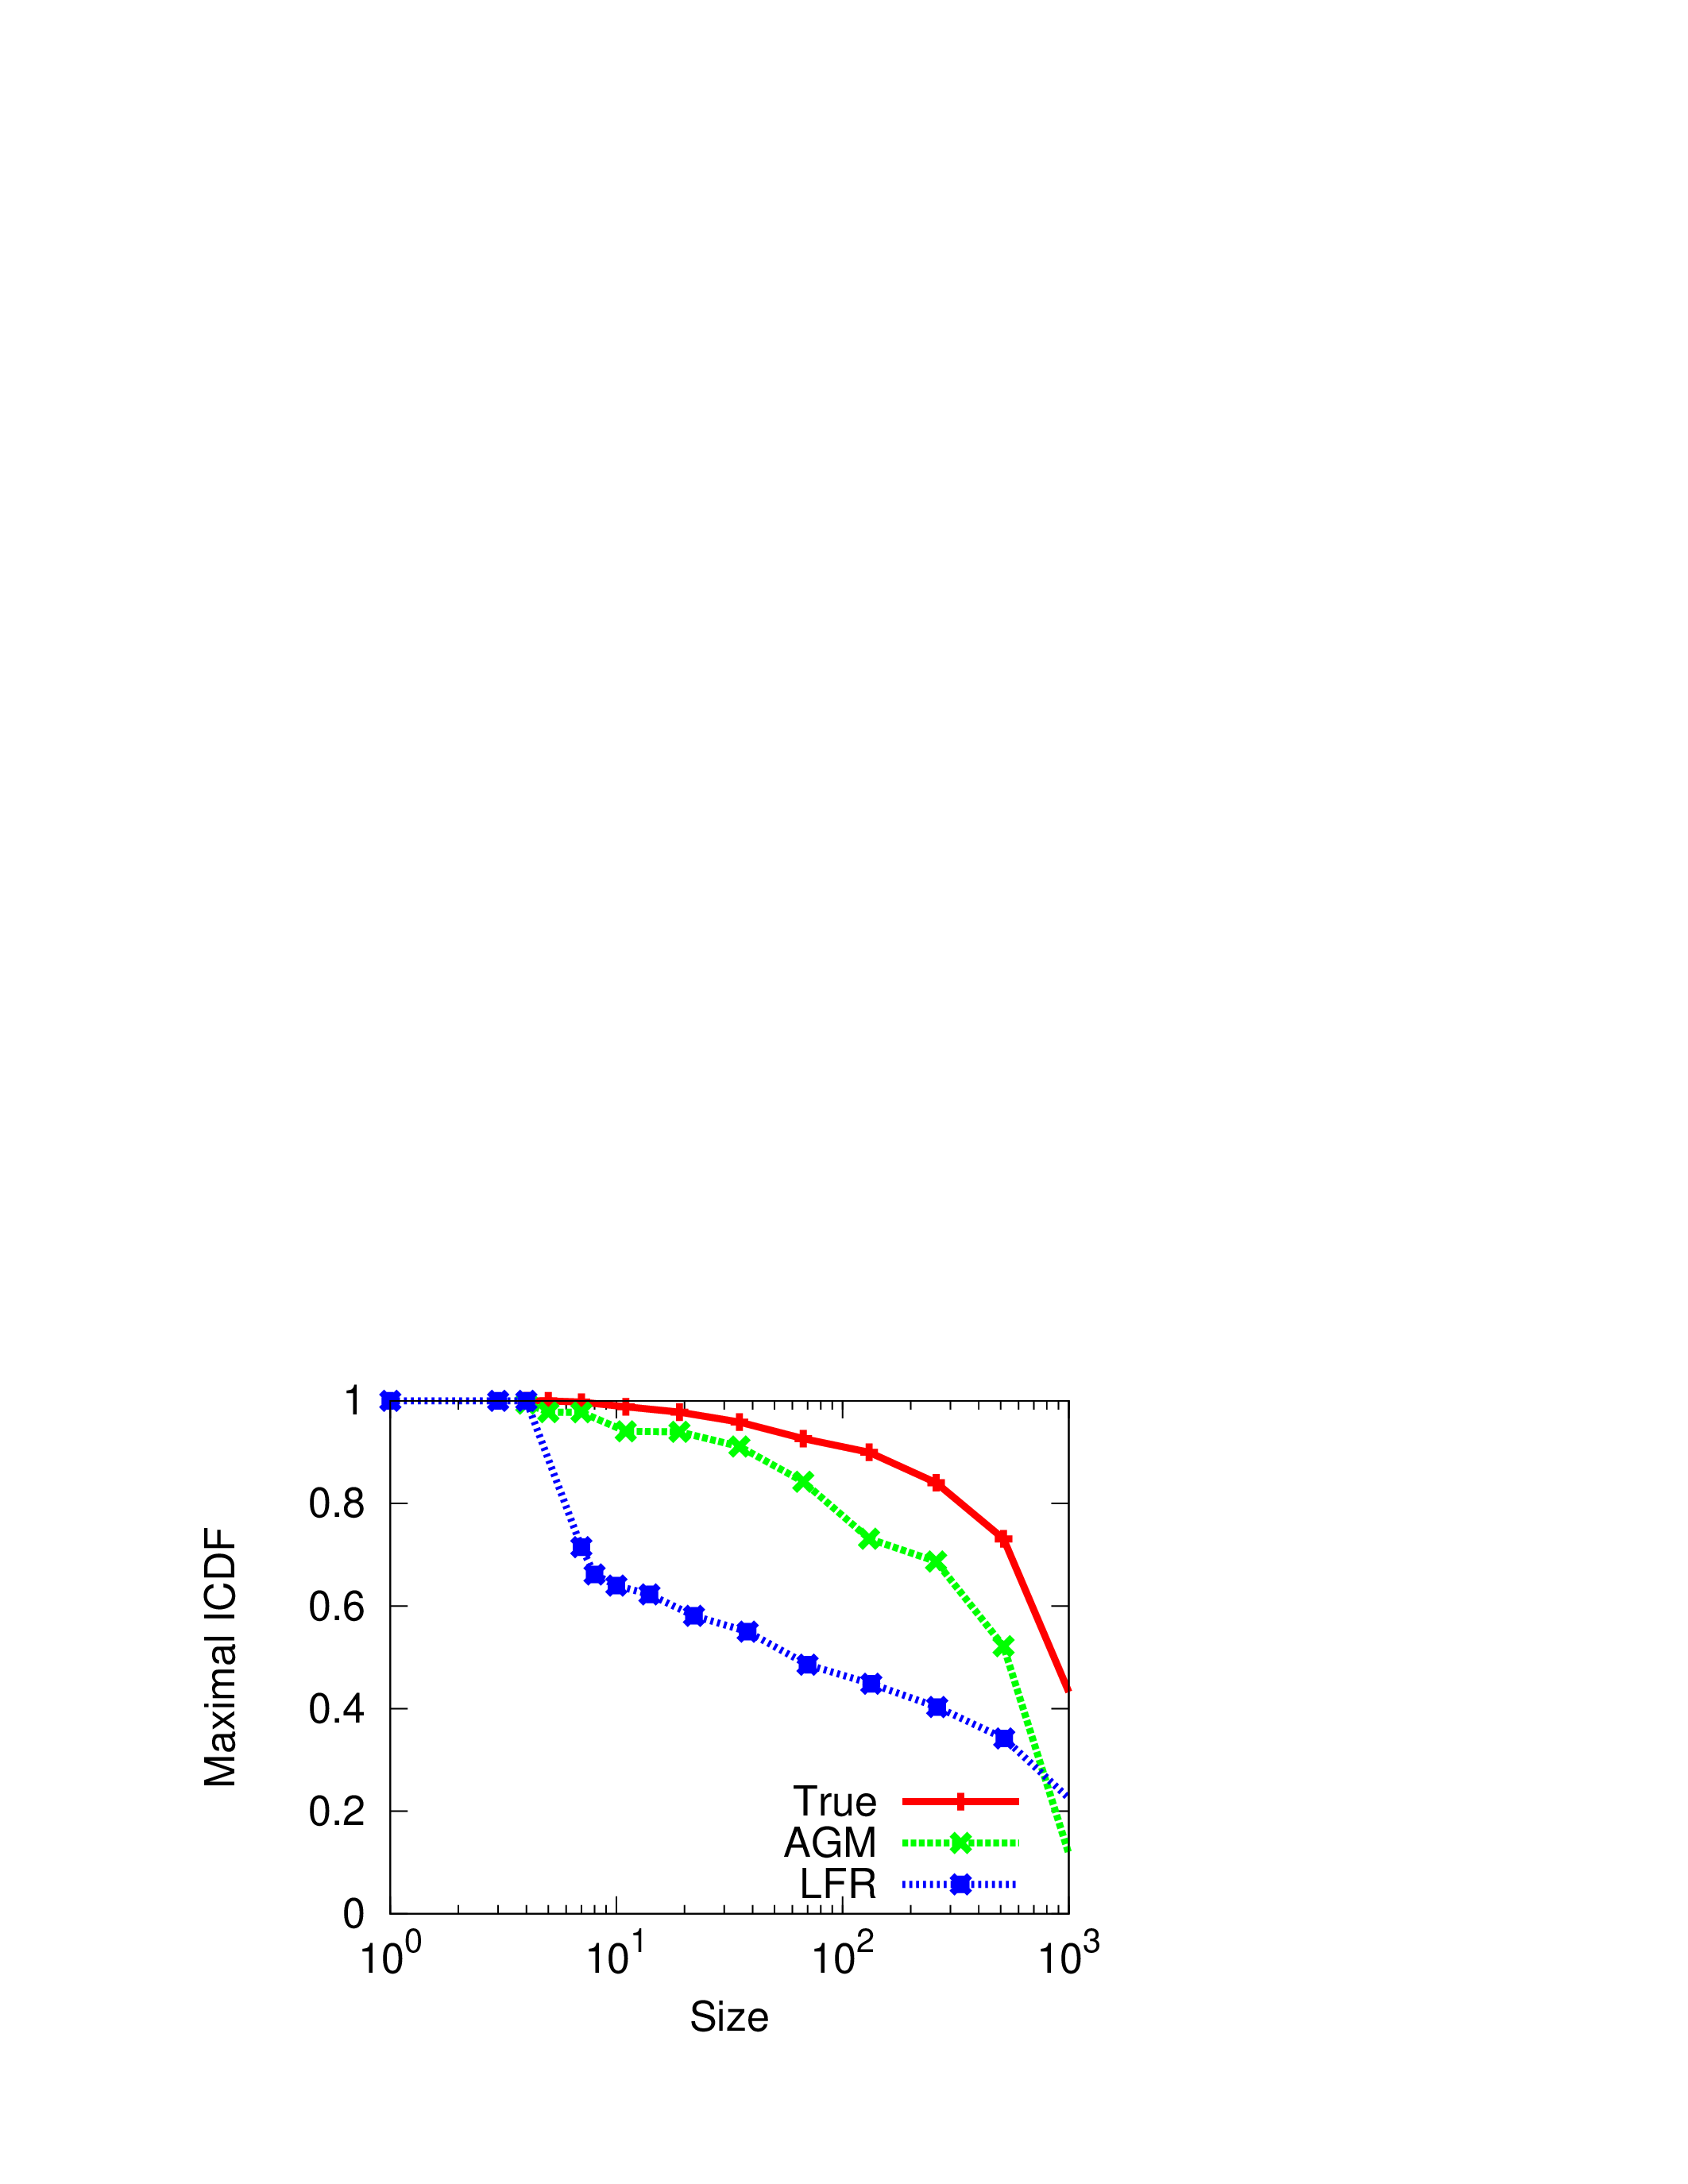}}
	\subfigure[Maximum ICDF	 (Friendster)]{\includegraphics[width=0.16\textwidth]{Models.P.Sz.MaxIntDeg.friendster.eps}}
	\subfigure[Maximum ICDF	 (Orkut)]{\includegraphics[width=0.16\textwidth]{Models.P.Sz.MaxIntDeg.orkut.eps}}
	\subfigure[Maximum ICDF	 (DBLP)]{\includegraphics[width=0.16\textwidth]{Models.P.Sz.MaxIntDeg.dblp.eps}}
	\subfigure[Maximum ICDF	 (IMDB)]{\includegraphics[width=0.16\textwidth]{Models.P.Sz.MaxIntDeg.imdbc.eps}}
	\subfigure[Maximum ICDF	 (Amazon)]{\includegraphics[width=0.16\textwidth]{Models.P.Sz.MaxIntDeg.amazon.eps}}
	\caption{Model comparison: Group properties.}
\label{fig:Full.Models.Groupstats}
\end{figure*}

\begin{figure*}[t]
	\centering
	\subfigure[LJ]{\includegraphics[width=0.16\textwidth]{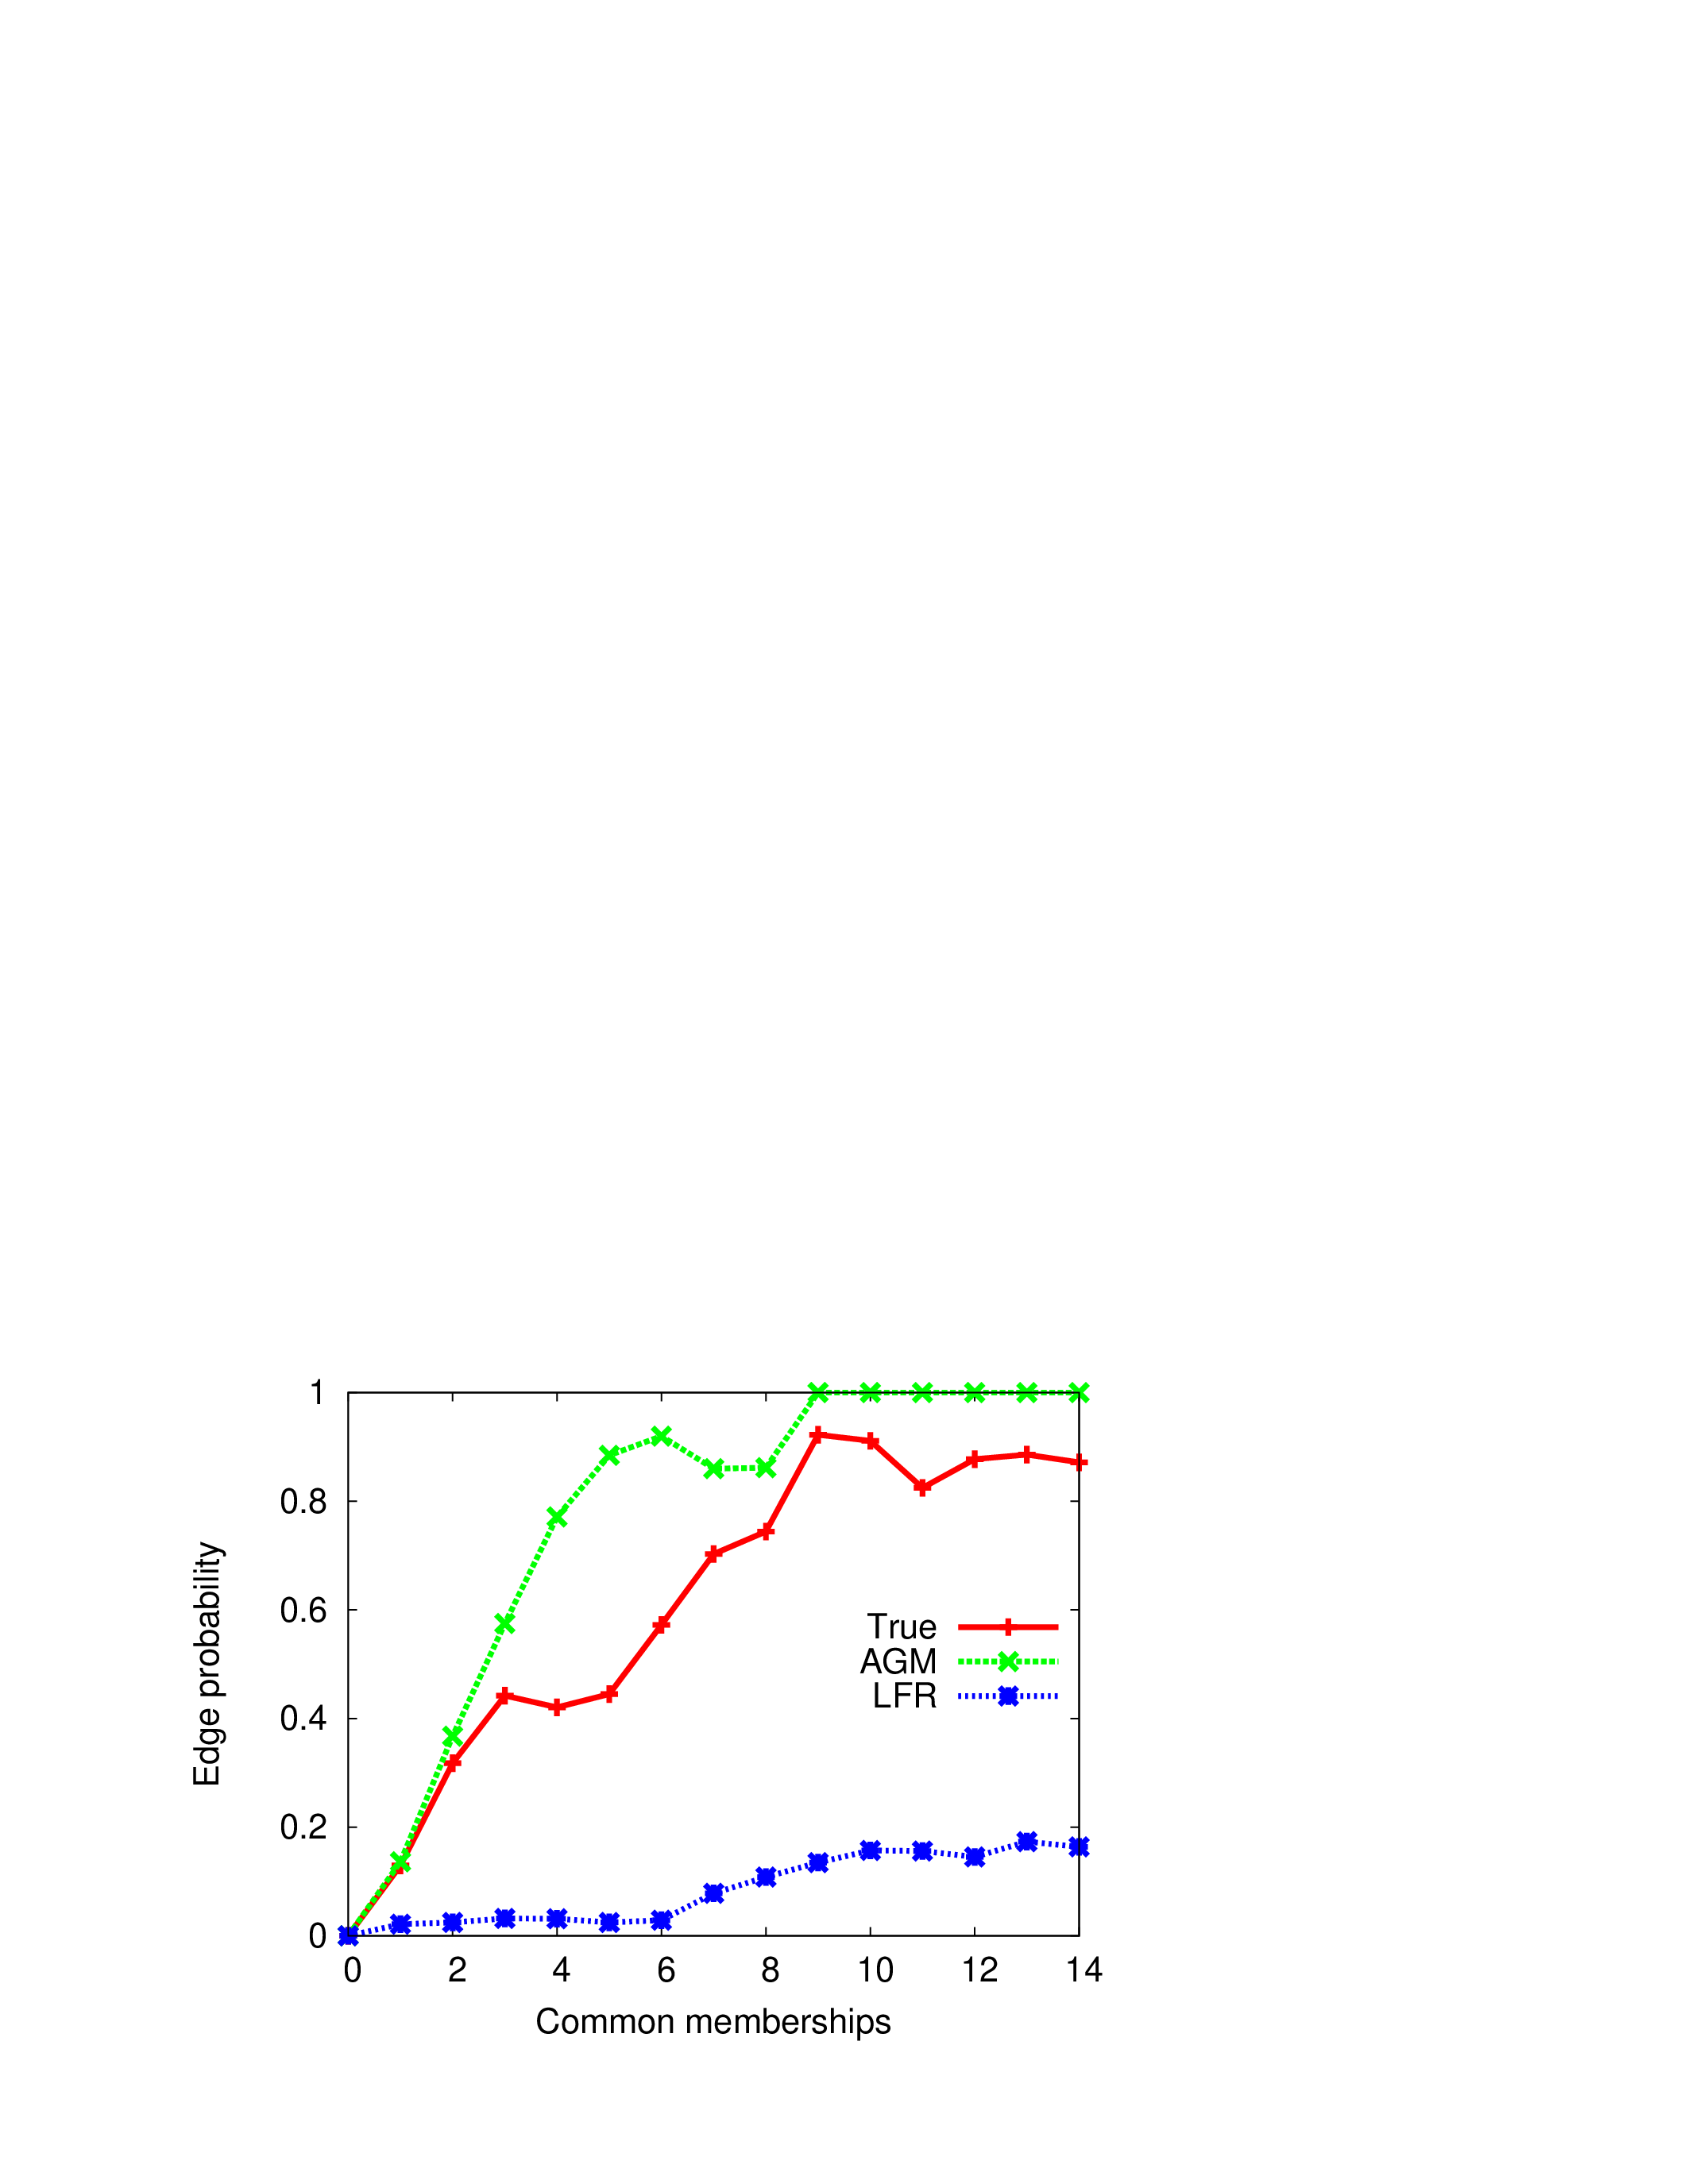}}
	 \subfigure[Friendster]{\includegraphics[width=0.16\textwidth]{Models.P.EdgeProb.friendster.eps}}
	\subfigure[Orkut]{\includegraphics[width=0.16\textwidth]{Models.P.EdgeProb.orkut.eps}}
	\subfigure[DBLP]{\includegraphics[width=0.16\textwidth]{Models.P.EdgeProb.dblp.eps}}
	\subfigure[IMDB]{\includegraphics[width=0.16\textwidth]{Models.P.EdgeProb.imdbc.eps}}
	 \subfigure[Amazon]{\includegraphics[width=0.16\textwidth]{Models.P.EdgeProb.amazon.eps}}
	\caption{Model comparison: Conditional edge probability between two nodes given the number
 of common groups that they belong to.}
\label{fig:Full.Models.edge_prob}
\end{figure*}

\begin{figure*}[t]
	\centering
	 \subfigure[LJ]{\includegraphics[width=0.16\textwidth]{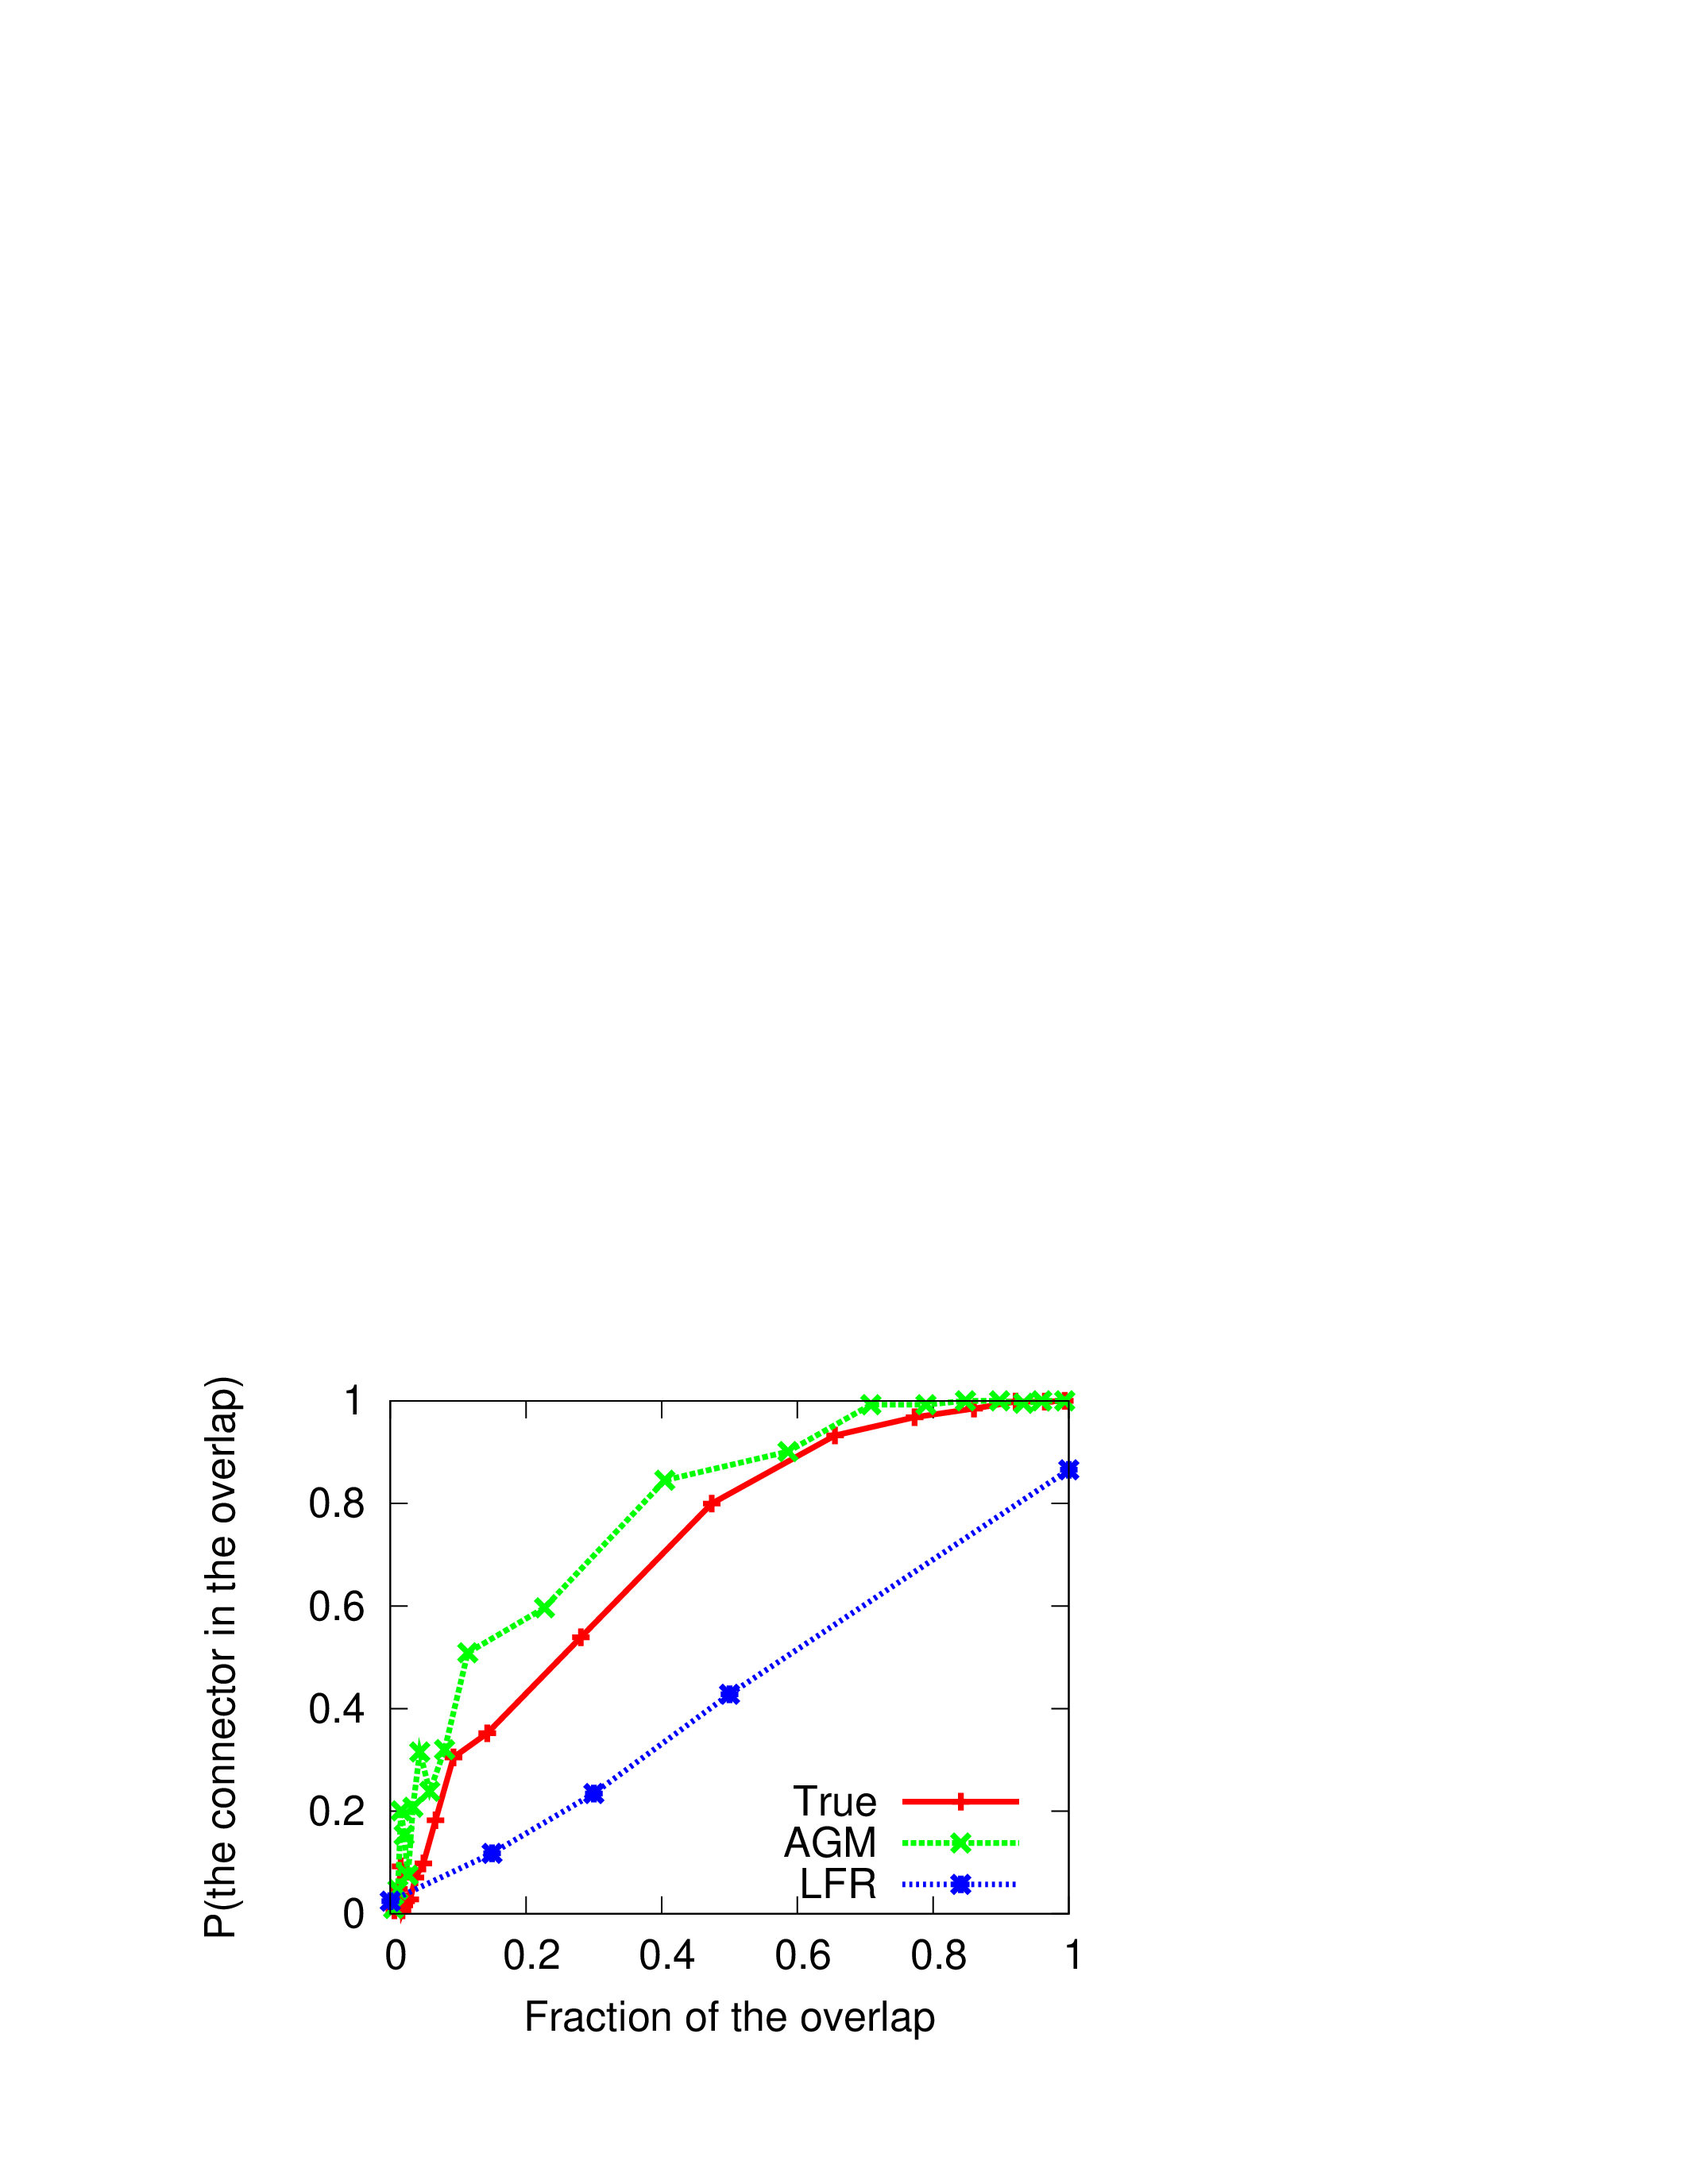}}
	 \subfigure[Friendster]{\includegraphics[width=0.16\textwidth]{Models.P.OlpFrac.HubInOlp.friendster.eps}}
	 \subfigure[Orkut]{\includegraphics[width=0.16\textwidth]{Models.P.OlpFrac.HubInOlp.orkut.eps}}
	 \subfigure[DBLP]{\includegraphics[width=0.16\textwidth]{Models.P.OlpFrac.HubInOlp.dblp.eps}}
	 \subfigure[IMDB]{\includegraphics[width=0.16\textwidth]{Models.P.OlpFrac.HubInOlp.imdbc.eps}}
	 \subfigure[Amazon]{\includegraphics[width=0.16\textwidth]{Models.P.OlpFrac.HubInOlp.amazon.eps}}
	\caption{Model comparison: Probability of a hub node belonging to the overlap as a function of the fraction of the overlap size to the group size.}
\label{fig:Full.hub.overlap.models}
\end{figure*}

\hide{
\begin{figure}[t]
\centering
  \subfigure[Edges inside the group]{\includegraphics[width=0.23\textwidth]{Rnd.Sz.Vol.eps}}
  \subfigure[Maximum internal degree]{\includegraphics[width=0.23\textwidth]{Rnd.Sz.MaxIntDeg.eps}}
  \caption{Edges inside the group and Maximum internal degree as a function of the group size.}
\end{figure}

\begin{figure}[t]
\centering
  \subfigure[Average IDF]{\includegraphics[width=0.23\textwidth]{Rnd.Sz.AvgIDF.eps}}
  \subfigure[The IDF of a connector]{\includegraphics[width=0.23\textwidth]{Rnd.Sz.HubIDF.eps}}
  \caption{In-degree fraction (IDF) as a function of the group size.}
\end{figure}
\begin{figure*}[t]
	\centering
	\subfigure[LJ]{\includegraphics[width=0.31\textwidth]{Rnd.OverlapCCF.lj.eps}}
	\subfigure[Ning]{\includegraphics[width=0.31\textwidth]{Rnd.OverlapCCF.Ning.eps}}
	\subfigure[Amazon]{\includegraphics[width=0.31\textwidth]{Rnd.OverlapCCF.amazon.eps}}
	\subfigure[DBLP]{\includegraphics[width=0.31\textwidth]{Rnd.OverlapCCF.dblp.eps}}
	\subfigure[imdbc]{\includegraphics[width=0.31\textwidth]{Rnd.OverlapCCF.imdbc.eps}}
	 \subfigure[Friendster]{\includegraphics[width=0.31\textwidth]{Rnd.OverlapCCF.friendster.eps}}
	\caption{The fraction of connected pairs of neighbors. AABB: both neighbors in either A or B, OO: both neighbors in O, AB: one neighbor in A and the other in B (or vice versa).}
\end{figure*}

\begin{figure}[t]
\centering
  \centering
  \epsfig{file=Rnd.OlpFrac.HubInOlp.eps, width=0.8\linewidth}
  \vspace{-5mm}
  \caption{Probability of a connector node belonging to the group overlap as a function of
  the fraction of group members in the overlap.}
  \vspace{-5mm}
\end{figure}

\begin{figure*}[t]
	\centering
	\subfigure[LJ]{\includegraphics[width=0.31\textwidth]{Rnd.EdgeProb.lj.eps}}
	\subfigure[Ning]{\includegraphics[width=0.31\textwidth]{Rnd.EdgeProb.Ning.eps}}
	\subfigure[Amazon]{\includegraphics[width=0.31\textwidth]{Rnd.EdgeProb.amazon.eps}}
	\subfigure[DBLP]{\includegraphics[width=0.31\textwidth]{Rnd.EdgeProb.dblp.eps}}
	\subfigure[imdbc]{\includegraphics[width=0.31\textwidth]{Rnd.EdgeProb.imdbc.eps}}
	 \subfigure[Friendster]{\includegraphics[width=0.31\textwidth]{Rnd.EdgeProb.friendster.eps}}
	\caption{Conditional edge probability between two nodes given the number
 of common groups that they belong to.}
\end{figure*}

\begin{table}[t]
\centering
  \begin{tabular}{c||c|c|c|c}
        Model&Degree&TP&SngVal&SngVec\\ \hline \hline
		AGM&2.23&2.48&1.52&1.17\\ \hline
		LFR&1.43&2.72&1.22&1.64
  \end{tabular}
  \caption{PowerKS statistics (Fitting, NOT POWER LAW)}
  \label{table:ks.network}
\end{table}

\begin{table}[t]
\centering
  \begin{tabular}{c||c|c|c|c|c|c}
        Model&Vol&MaxDeg&HubProb&EdgeProb&OO&AABB\\ \hline \hline
		AGM&0.03&0.26&0.20&0.50&0.25&0.44\\ \hline
		LFR&0.06&0.15&0.50&0.67&0.60&0.59
\end{tabular}
  \caption{PowerKS statistics for Group and overlap statistics (Fitting, NOT POWER LAW)}
  \label{table:ks.group}
\end{table}

\begin{figure}[t]
\centering
  \epsfig{file=Grouppdf.eps, width=0.7\linewidth}
  \vspace{-5mm}
  \caption{Size distribution of three sets of groups in the data sets}
  \label{fig:group_sz}
  \vspace{-7mm}
\end{figure}

\begin{figure}[t]
  \centering
  \subfigure[Conductance]{\includegraphics[width=0.23\textwidth]{Sz.Phi.eps}}
  \subfigure[Modularity]{\includegraphics[width=0.23\textwidth]{Sz.Modularity.eps}}
  \subfigure[Expansion]{\includegraphics[width=0.23\textwidth]{Sz.Expansion.eps}}
  \subfigure[Average Internal Degree]{\includegraphics[width=0.23\textwidth]{Sz.AvgDeg.eps}}
  \caption{Group properties as a function of group size. Modularity and Average Internal
  Degree increases as a group becomes larger. Both conductance and expansion are very high.}
  \label{fig:Metric_All}
\end{figure}

%\begin{figure}[h]
%\centering
%  \centering
%  \subfigure[Conductance(LC)/Conductance]{\includegraphics[width=0.23\textwidth]{Sz.BestPhiOrigPhi.eps}}
%  \subfigure[Recall(LC)]{\includegraphics[width=0.23\textwidth]{Sz.RecallLC.eps}}
%  \subfigure[Precision(LC)]{\includegraphics[width=0.23\textwidth]{Sz.PrecisionLC.eps}}
%  \subfigure[Distance in the Whole Graph/Distance in the Group]{\includegraphics[width=0.23\textwidth]{Sz.DistInOut.eps}}
%  \subfigure[Best Internal Conductance/Conductance]{\includegraphics[width=0.23\textwidth]{Sz.PhiInOut.eps}}
%  \caption{Group statistics}
%  \label{fig:groupstat.appendix}
%\end{figure}
\subsection{Community scores}

\xhdr{Description of community scores that we used} Let $G(V,E)$ be an undirected graph with $n = |V |$
nodes and $m = |E|$ edges. Let $S$ be the set of nodes in the cluster, where
$n_S$ is the number of nodes in $S$, $n_S = |S|$; $m_S$ the number of edges in
$S$, $m_S = |{(u, v) : u 2 S, v 2 S}|$; and $c_S$, the number of edges on the
boundary of $S$, $c_S = |{(u, v) : u 2 S, v 62 S}|$; and $d(u)$ is the degree
of node $u$. We consider the following 13 metrics $f(S)$ that capture the
notion of a quality of the cluster.
%Lower value of score $f(S)$ (when $|S|$ is kept constant) suggests that $S$ is more community-like.

\begin{itemize}
  \denselist
  \item Conductance: $f(S) = \frac{c_S}{2m_S+c_S}$ measures the fraction of
      total edge volume that points outside the cluster.
  \item Expansion: $f(S) = \frac{c_S}{n_S}$ measures the number of edges
      per node that point outside the cluster.
  \item Internal density: $f(S) = 1-\frac{m_S}{n_S(n_S-1)/2}$) is the
      internal edge density of the cluster $S$.
  \item Cut Ratio: $f(S) = \frac{c_S}{n_S(n-n_S)}$) is the fraction of all
      possible edges leaving the cluster.
  \item Normalized Cut: $f(S) = \frac{c_S}{2m_S+c_S} + \frac{c_S}{2(m-m_S)+c_S}$)
  \item Maximum-ODF (Out Degree Fraction): $f(S) = \max_{u \in S}
      \frac{|\{(u,v):v \not\in S\}|}{d(u)}$) is the maximum fraction of
      edges of a node pointing outside the cluster.
  \item Average-ODF: $f(S) = \frac{1}{n_S} \sum_{u \in S}\frac{|\{(u,v):v
      \not\in S\}|}{d(u)}$) is the average fraction of nodes' edges
      pointing outside the cluster.
  \item Flake-ODF: \\$f(S) = \frac{|\{u:u \in S,|\{(u,v):v \in
      S\}|<d(u)/2\}|}{n_S}$ is the fraction of nodes in S that have fewer
      edges pointing inside than to the outside of the cluster.
  \item Modularity: $f(S) = \frac{1}{4} (m_S - E(m_S))$ ($E(m_S)$ is the
      expected number of edges between the nodes in set S in a random graph
      with the same node degree sequence.)
  \item Edges Inside: $f(S) = m_S$ is the number of edges between the
      members of $S$.
  \item Average Degree:$f(S) = \frac{2 m_S}{n_S}$ is the average internal degree
        of the members of $S$.
  \item Fraction Over Median Degree (FOMD): \\
  $f(S) = \frac{|\{u:u \in S, |\{(u,v):v \in S\}| > d_m\}|}{n_S}$
        is the fraction of member nodes of $S$ that have internal degrees higher than
        $d_m$, where $d_m$ is the median value of $d(u)$ of all nodes in the entire graph (all $u \in V$).
  \item Triangle Participation Ratio (TPR): \\
  $f(S) = \frac{|\{u:u \in S, \{(v,w):v,w \in S, (u,v) \in E, (u,w) \in E, (v,w) \in E\} \neq \varnothing\}|}{n_S}$
  is the fraction of member nodes that belong
      to at least one triad.
  %. Edges cut: cS is number of edges needed to be removed to
  %disconnect nodes in S from the rest of the network.
  %is the
  %fraction of nodes in S that have fewer edges pointing inside
  %than to the outside of the cluster [10].
\end{itemize}

We assume that some of the scores would be highly correlated one another and
therefore it is not a good idea to use all the scores. If one score is
correlated to many other scores, then using all scores will be in fact same as
measuring the score multiple times. Therefore, we first measured the
relationship between 13 scores. We evaluated 13 scores for the 30,000 groups in
LiveJournal and computed the correlation coefficient between each pair of
scores. If the correlation coefficient of a pair of scores is above a
threshold, we made an edge between the scores. In this way, we constructed a
relationship graph among 13 scores in Figure~\ref{fig:graph_scores}. We can see
two large clusters and two small clusters of scores. The largest cluster
contains the scores about the internal connectivity of a group (Internal
Density, Average Degree, FOMD, TPA, Edges Inside). The scores in the other
large cluster measure the ratio between the internal and external connectivity
of a group (Flake-ODF, Conductance, Average ODF, Maximum ODF, Normalized Cut)
Also we find a small cluster about the scores measuring the external
connectivity (CutRatio, Expansion), and finally we find a singleton cluster of
modularity. From these clusters, we select 6 scores -- FOMD, TPA, Conductance,
Flake-ODF, Cut Ratio, Modularity --, two scores from each of large clusters,
and one score from each of small clusters.

After choosing a set of scores, the question becomes how to aggregate different
scores as each score varies in its scale. Here, we are interested in ordering
groups rather than measuring the absolute value of aggregated scores. For each
score, we ordered groups by the score and record the rank of each group. In
this way, each group had 6 ranks for each score. Then, we found the median rank
of each group, and consider it as a new score, namely ''average rank''. We
ordered groups by their average rank and chose the best $k$ groups by average
rank. To validate that this average rank is a reliable way to choose groups
with desirable properties, we conduct the following experiment. Given a score
$i$, we choose top $k$ groups by the score, and we measure the average values
of a property $g$ and denote the average value by $f_i(k)$. In
Figure~\ref{fig:rank.AvgPath}, we use 6 different $f$'s:  the average shortest
path length between two nodes in a community, and so on.
Figure~\ref{fig:rank.AvgPath} shows that sorting groups by the average rank
results in good average value of the selected groups for all the properties
that we measured.
%It is because modularity has a resolution limit, and prefers bigger communities.
%Next question is how many communities we would choose. We choose 5,000 communities. (To be added)

\begin{figure}[t]
\centering
  \epsfig{file=graph_scores.eps, width=0.7\linewidth}
  \caption{Relation among scores. Scores are connected if their correlation coefficient is over 0.59}
  \label{fig:graph_scores}
\end{figure}

%%%%%%%%%%%%%%
%% THIS CAN GO!

\begin{figure}[t]
  \centering
  \epsfig{file=rank_property.eps, width=0.9\linewidth}
  \caption{
  Average metrics of top $\bf k$ communities in LiveJournal and Ning
  ranked using different notions of community quality.}
  %See the main text for the description of scores.}
  \label{fig:rank_property}
\end{figure}

\xhdr{Group score comparison} Figure~\ref{fig:rank_property} shows the various properties
that we hypothesize community like groups of nodes would have. For example, a
set of nodes is a good community if the average network shortest path between
the members of the community is short (separability), number of edges (density)
and clustering coefficient (CCF) among the members is large, and internally
communities are cohesive (one has to cut many edges between the community can
be split). For each group we compute a score (modularity, conductance, TPR),
rank the groups by score and then plot the average metric over the top $k$
groups. Notice poor performance of modularity -- it prefers groups of low
density, low clustering coefficient and cohesiveness as well as separability.
On the other hand metrics like conductance and triad participation ratio (TPR)
perform much better as top ranked groups are good communities in a sense that
they are dense, have high clustering coefficient, are internally cohesive and
have low separation between their members.

%
%\begin{figure}[t]
%  \centering
%  \subfigure[Edges Inside/Cut (LJ)]{\includegraphics[width=0.23\textwidth]{rank_property.CutToEdgeIns.lj.eps} \label{xx}}
%  \subfigure[Edges Inside/Cut (Ning)]{\includegraphics[width=0.23\textwidth]{rank_property.CutToEdgeIns.NingL.eps}}
%  \subfigure[Density (LJ)]{\includegraphics[width=0.23\textwidth]{rank_property.Density.lj.eps}}
%  \subfigure[Density (Ning)]{\includegraphics[width=0.23\textwidth]{rank_property.Density.NingL.eps}}
%  \subfigure[Cohesiveness (LJ)]{\includegraphics[width=0.23\textwidth]{rank_property.InsidePhi.lj.eps}}
%  \subfigure[Cohesiveness (Ning)]{\includegraphics[width=0.23\textwidth]{rank_property.InsidePhi.NingL.eps}}
%  \subfigure[CCF (LJ)]{\includegraphics[width=0.23\textwidth]{rank_property.CCF.lj.eps}}
%  \subfigure[CCF (Ning)]{\includegraphics[width=0.23\textwidth]{rank_property.CCF.NingL.eps}}
%  \caption{Average metrics of top k communities in LiveJournal and Ning by 7 scores. See the main text for the description of scores}
%  \label{fig:rank.AvgPath}
%\end{figure}

\subsection{Parameter selection for LFR}
In Section\ref{sec:model}, we generated synthetic graphs by our AGM model and the LFR model, and
compared the properties of groups in two synthetic graphs.
We use the \cag of the LiveJournal network $B_{LJ}(V,B,E)$ as an input for both models.
In this section, we describe how we choose other parameters for the models.

AGM requires only one additional parameter, $\alpha$ and we can estimate $\alpha$ from Figure~\ref{fig:sz.vol}.
In AGM, the number of edges $m_S$ inside the group $S$ that has $n_S$ member nodes is proportional to
$n_S^{2-\alpha}$. We observe that $m_S \propto n_S^1.6$ in Figure~\ref{fig:sz.vol} in LiveJournal,
and therefore set $\alpha=0.4$.

LFR requires the power law coefficient $\gamma$ of node degree distribution  and the mixing parameter $\mu$.
From the LiveJournal graph, we take the nodes $V_g$ that belong to at least one group, and take the induced subgraph
$G(V_g,E_g)$ of these nodes. We fit $\gamma$ and $\mu$ from $G(V_g,E_g)$. We used $\gamma = -1.5$ and $\mu=0.1$.
$1-\mu$ is the average in-degree fraction in Figure\ref{fig:sz.avgidf}. From Figure~\ref{fig:sz.avgidf},
one might think that we should use $\mu$ about 0.4. However, the average in-degree fraction in Figure~\ref{fig:sz.avgidf}
is measured in the entire graph $G(V,E)$. Since we use LFR to generate $G(V_g,E_g)$, we measure the average in-degree fraction in $G(V_g,E_g)$
and it suggests $\mu$ is about $0.1$. We tested over different values of $\mu$ and $\gamma$ around our choice and found that the results
are similar.

\begin{figure}[t]
  \centering
  \epsfig{file=Mempdf.LJ.eps, width=0.6\linewidth}
  \caption{
  The distribution of the membership size of nodes (how many groups a node belongs to)
  with 5,000 LiveJournal groups.
    The distribution seems to follow a power law with cut-off on the maximum.
    }
  %See the main text for the description of scores.}
  \label{fig:mem.size}
\end{figure}
\clearpage

%%%%
%%Previously used plots
%\begin{figure}[t]
%\centering
%  \centering
%  \subfigure[LJ]{\includegraphics[width=0.23\textwidth]{node.Deg.CCF.lj.eps}}
%  \subfigure[Ning]{\includegraphics[width=0.23\textwidth]{node.Deg.CCF.NingL.eps}}
%  \vspace{-5mm}
%  \caption{The clustering coefficient (CCF) of non-memberhip nodes, single-membership nodes, and multi-membership nodes.}
%  \label{fig:Overlap.CCF}
%  \vspace{-4mm}
%\end{figure}
%
%\begin{figure*}[t]
%	\centering
%	\subfigure[LJ]{\includegraphics[width=0.185\textwidth]{node.Deg.CCF.lj.eps}}
%	\subfigure[Ning]{\includegraphics[width=0.185\textwidth]{node.Deg.CCF.Ning.eps}}
%	\subfigure[Amazon]{\includegraphics[width=0.185\textwidth]{node.Deg.CCF.amazon.eps}}
%	\subfigure[DBLP]{\includegraphics[width=0.185\textwidth]{node.Deg.CCF.dblp.eps}}
%	\subfigure[IMDB]{\includegraphics[width=0.185\textwidth]{node.Deg.CCF.imdbc.eps}}
%	\caption{The clustering coefficient (CCF) of non-memberhip nodes, single-membership nodes, and multi-membership nodes.}
%\label{fig:Full.Overlap.CCF}
%\end{figure*}

\subsection{Model Comparison in Ning}
\begin{figure}[h]
\centering
  \centering
  \subfigure[Effective Diameter]{\label{fig:sz.effdiam.models.Ning}\includegraphics[width=0.23\textwidth]{Sz.EffDIam.Models.Ning.eps}}
  \subfigure[Edges Inside the group]{\label{fig:sz.vol.models.Ning}\includegraphics[width=0.23\textwidth]{Sz.Vol.Models.Ning.eps}}
  \subfigure[Maximum internal degree]{\label{fig:sz.hub.models.Ning}\includegraphics[width=0.23\textwidth]{Sz.Hub.Models.Ning.eps}}
  \subfigure[Average path length]{\label{fig:sz.avgpath.models.Ning}\includegraphics[width=0.23\textwidth]{Sz.AvgPath.Models.Ning.eps}}
  \vspace{-5mm}
  \caption{Model comparison (Ning): Ning group properties.}
  \vspace{-5mm}
  \label{fig:group.stat.models}
\end{figure}

\begin{figure}[h]
\centering
  \centering
  \subfigure[Single Membership]{\label{fig:Overlap.CCF.AGM.Ning}\includegraphics[width=0.23\textwidth]{node.Deg.CCF.Single.Ning.eps}}
  \subfigure[Multi Membership]{\label{fig:Overlap.CCF.LFR.Ning}\includegraphics[width=0.23\textwidth]{node.Deg.CCF.Double.Ning.eps}}
  \vspace{-5mm}
  \caption{Model comparison (Ning): Clustering coefficient (CCF) of single-membership nodes and
  multi-membership nodes.}
  \vspace{-5mm}
  \label{fig:Overlap.CCF.Models}
\end{figure}

\begin{figure}[h]
\centering
  \centering
  \subfigure[AGM]{\label{fig:Overlap.Triangle.AGM.Ning}\includegraphics[width=0.23\textwidth]{OverlapCCF.AGM1.Ning.eps}}
  \subfigure[LFR]{\label{fig:Overlap.Triangle.LFR.Ning}\includegraphics[width=0.23\textwidth]{OverlapCCF.LFR.Ning.eps}}
  \vspace{-5mm}
  \caption{Model comparison (Ning): The fraction of connected pairs of neighbors that are either in A or B (AABB), or in O (OO).}
  \label{fig:Overlap.Triangle.Models}
  \vspace{-5mm}
\end{figure}

\begin{figure}[h]
\centering
  \centering
  \subfigure[Fraction of the overlap size]{\label{fig:Overlap.Hub.OVF.Ning}\includegraphics[width=0.23\textwidth]{OlpFrac.HubInOlp.Models.Ning.eps}}
  \subfigure[Overlap size]{\label{fig:Overlap.Hub.OvSz.Ning}\includegraphics[width=0.23\textwidth]{OlpSz.HubInOlp.Models.Ning.eps}}
  \vspace{-5mm}
  \caption{Model comparison (Ning): Probability of a hub node belonging to the overlap as a function of (a) the fraction of the overlap size to the group size, (b) the overlap size.}
  \label{fig:hub.overlap.models}
  \vspace{-5mm}
\end{figure}

\begin{figure}[h]
\centering
  \includegraphics[width=0.4\textwidth]{EdgeProb.Models.Ning.eps}
  \vspace{-5mm}
  \caption{Model comparison (Ning):Edge probability versus common membership}
  \vspace{-5mm}
\end{figure}

\clearpage
\subsection{Model comparison with synthetic group memberships}
\begin{figure}[h]
\centering
  \centering
  \subfigure[Effective Diameter]{\label{fig:sz.effdiam.models.Synthetic}\includegraphics[width=0.23\textwidth]{Sz.EffDIam.Models.Synthetic.eps}}
  \subfigure[Edges Inside the group]{\label{fig:sz.vol.models.Synthetic}\includegraphics[width=0.23\textwidth]{Sz.Vol.Models.Synthetic.eps}}
  \subfigure[Maximum internal degree]{\label{fig:sz.hub.models.Synthetic}\includegraphics[width=0.23\textwidth]{Sz.Hub.Models.Synthetic.eps}}
  \subfigure[Average path length]{\label{fig:sz.avgpath.models.Synthetic}\includegraphics[width=0.23\textwidth]{Sz.AvgPath.Models.Synthetic.eps}}
  \vspace{-5mm}
  \caption{Model comparison (Synthetic): Synthetic group properties.}
  \vspace{-5mm}
  \label{fig:group.stat.models}
\end{figure}

\begin{figure}[h]
\centering
  \centering
  \subfigure[Single Membership]{\label{fig:Overlap.CCF.AGM.Synthetic}\includegraphics[width=0.23\textwidth]{node.Deg.CCF.Single.Synthetic.eps}}
  \subfigure[Multi Membership]{\label{fig:Overlap.CCF.LFR.Synthetic}\includegraphics[width=0.23\textwidth]{node.Deg.CCF.Double.Synthetic.eps}}
  \vspace{-5mm}
  \caption{Model comparison (Synthetic): Clustering coefficient (CCF) of single-membership nodes and
  multi-membership nodes.}
  \vspace{-5mm}
  \label{fig:Overlap.CCF.Models}
\end{figure}

\begin{figure}[h]
\centering
  \centering
  \subfigure[AGM]{\label{fig:Overlap.Triangle.AGM.Synthetic}\includegraphics[width=0.23\textwidth]{OverlapCCF.AGM1.Synthetic.eps}}
  \subfigure[LFR]{\label{fig:Overlap.Triangle.LFR.Synthetic}\includegraphics[width=0.23\textwidth]{OverlapCCF.LFR.Synthetic.eps}}
  \vspace{-5mm}
  \caption{Model comparison (Synthetic): The fraction of connected pairs of neighbors that are either in A or B (AABB), or in O (OO).}
  \label{fig:Overlap.Triangle.Models}
  \vspace{-5mm}
\end{figure}

\begin{figure}[h]
\centering
  \centering
  \subfigure[Fraction of the overlap size]{\label{fig:Overlap.Hub.OVF.Synthetic}\includegraphics[width=0.23\textwidth]{OlpFrac.HubInOlp.Models.Synthetic.eps}}
  \subfigure[Overlap size]{\label{fig:Overlap.Hub.OvSz.Synthetic}\includegraphics[width=0.23\textwidth]{OlpSz.HubInOlp.Models.Synthetic.eps}}
  \vspace{-5mm}
  \caption{Model comparison (Synthetic): Probability of a hub node belonging to the overlap as a function of (a) the fraction of the overlap size to the group size, (b) the overlap size.}
  \label{fig:hub.overlap.models}
  \vspace{-5mm}
\end{figure}

}
